# Supplementary material for: A Simple Graph Contrastive Learning Framework for Short Text Classification
Source: arXiv:2501.09219 source file (2025-01-16)
Supplement: Supplementary file 1 [file appendix.tex]

\section{Appendix}
\subsection{A.1 Illustration of Multi-View Graph Construction}
\label{construction}
We present a toy example of multi-view graph in Fig. \ref{toy}.
Note that %the solid lines represent the connections between terms and texts, while 
the dashed lines represent the internal connections within the multi-view graph.

We first obtain words, entities, and POS tags from the corpus through tokenization, entity linking, and part-of-speech tagging, respectively. Then, we use fixed-size sliding windows on all texts in the corpus to collect co-occurrence statistics for words and POS tags separately to construct word-word and tag-tag edges. These edges are weighted by PMI, which are defined as follows:
\begin{equation}
\begin{aligned}
    &\text{PMI}(v_{\pi,i},v_{\pi,j})=\log\frac{I(v_{\pi,i},v_{\pi,i})}{I(v_{\pi,i})I(v_{\pi,i})}, \quad \pi\in\{w,p\}, \\
    &I(v_{\pi,i},v_{\pi,i}) = \frac{\Omega(v_{\pi,i},v_{\pi,i})}{\Omega}, \quad I(v_{\pi,i})= \frac{\Omega(v_{\pi,i})}{\Omega},
\end{aligned}
\end{equation}
where $\Omega(v_{\pi,i}, v_{\pi,j})$ is the number of sliding windows in the corpus that contain both node $v_{\pi,i}$ and node $v_{\pi,j}$, and $\Omega$ is the total number of sliding windows.

The rationale behind employing PMI for the construction of adjacency matrices $\mathbf{A}_w$ and $\mathbf{A}_p$ lies in PMI’s effectiveness as a popular measure of word associations, capturing local co-occurrence information between words within each text and the semantic relationships among those words. Furthermore, in TextGCN \cite{yao2019graph}, it has been observed that using PMI yields better results compared to using word count methods.

Due to the limited number of entities in short texts, it is not feasible to compute their co-occurrence. Alternatively, we compute the cosine similarity between each pair of entities and construct edges with a similarity greater than 0, \textit{i.e.}, $[\mathbf{A}_e]_{ij}=\text{max}(\cos(\mathcal{V}_{e,i},\mathcal{V}_{e,j}),0)$.

Next, we create edges between the text and nodes based on the occurrence of different types of nodes in the short text. The corresponding weight of each edge is determined by the TF-IDF approach.

\begin{figure}
    \centering
    \includegraphics[width=0.45\textwidth]{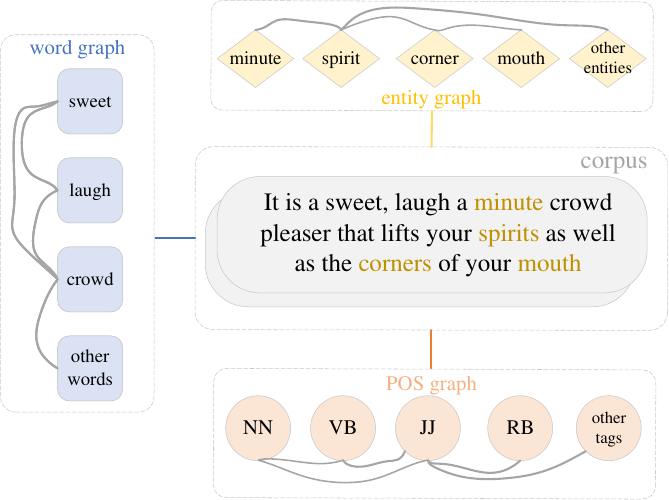}
    \caption{The toy example of multi-view graph construction, where rectangles represent words, diamonds represent entities, and circles represent POS tags. NN: noun, VB: verb, JJ: adjective, RB: adverb.}
    \label{toy}
\end{figure}

\subsection{A.2 Proof of Theorem}
\label{proof}
Before formal proof, We give the following notations. We consider a collection of $M$ views of short texts, denoted as $Z_1, \cdots, Z_M$. Actually, we use word-entity, entity-POS, and word-POS views in this work. For ease of presentation, we take two views $Z_1$ and $Z_2$ consisting of samples $\mathcal{Z}=\{\mathbf{Z}_1^i,\mathbf{Z}_2^j\}_{i,j=1}^N$ for example. The formed positive samples $(\mathbf{Z}_1^i, \mathbf{Z}_2^i)$ are drawn from a joint distribution $p(\mathbf{Z}_1, \mathbf{Z}_2)$, while the formed negative samples $(\mathbf{Z}_1^i, \mathbf{Z}_2^j)$ are drawn from the product of marginals $p(\mathbf{Z}_1)p(\mathbf{Z}_2)$. Let the discriminator be $f(\mathbf{Z}_1, \mathbf{Z}_2)=%\exp(\text{norm}(\Phi(\mathbf{Z}_1)),\text{norm}(\Phi(\mathbf{Z}_2))/\tau)=
\exp((\mathbf{Z}_1 \cdot \mathbf{Z}_2)/\tau)$.

Next, we present the following Lemma to connect the discriminator with the mutual information.
\begin{lemma}
\label{lemma_1}
    The discriminator $f$ is proportional to the density ratio of the joint distribution and the product of marginals, denoted as,
    $f(\mathbf{Z}_1,\mathbf{Z}_2) \propto \frac{p(\mathbf{Z}_1,\mathbf{Z}_2)}{p(\mathbf{Z}_1)p(\mathbf{Z}_2)}$.
\end{lemma}
\begin{proof}
    The CL loss essentially classifies the unique positive pairs from the formed paired data. Thus, for the $i$-th positive sample pair, we have,
    \begin{equation}
    \label{prop}
    \begin{aligned}
        p(\{\mathbf{Z}_1^i, \mathbf{Z}_2^i\}|\mathcal{Z})&=\frac{p(\mathbf{Z}_1^i,\mathbf{Z}_2^i)\Pi_{k=1,k\neq i}^Np(\mathbf{Z}_1^k)p(\mathbf{Z}_2^k)}{\sum_{j=0}^Np(\mathbf{Z}_1^j,\mathbf{Z}_2^j)\Pi_{k\neq j}p(\mathbf{Z}_1^k)p(\mathbf{Z}_2^k)} \\
        &\overset{(a)}{=}\frac{\frac{p(\mathbf{Z}_1^i,\mathbf{Z}_2^i)}{p(\mathbf{Z}_1^i)p(\mathbf{Z}_2^i)}}{\sum_{j=0}^N\frac{p(\mathbf{Z}_1^j,\mathbf{Z}_2^j)}{p(\mathbf{Z}_1^j)p(\mathbf{Z}_2^j)}}.
    \end{aligned}
    \end{equation}
\end{proof}
The equation (a) holds since we divide $\Pi_{k=0}^Np(\mathbf{Z}_1^k)p(\mathbf{Z}_2^k)$ for the numerator and denominator simultaneously. When comparing Eq.\ref{prop} with the CL loss, \textit{i.e.}, $-\log \frac{f(\mathbf{Z}_1^i,\mathbf{Z}_2^i)}{\sum_{j\in\mathcal{Z}}f(\mathbf{Z}_1^i, \mathbf{Z}_2^j)}$, we find that $f(\mathbf{Z}_1,\mathbf{Z}_2)$ is proportional to the $\frac{p(\mathbf{Z}_1,\mathbf{Z}_2)}{p(\mathbf{Z}_1)p(\mathbf{Z}_2)}$. Therefore, we complete the proof. 

Based on the Lemma \ref{lemma_1}, we begin to prove the Theorem 1. We can reformulate the CL loss with respect to views $Z_1$ and $Z_2$ as:
\begin{equation}
\label{mutual}
\begin{aligned}
    \mathcal{L}_{Z_1,Z_2}&=-\mathbb E_\mathcal{Z}\log\left[\frac{f(\mathbf{Z}_1^i,\mathbf{Z}_2^i)}{\sum_{j=0}^Nf(\mathbf{Z}_1^i,\mathbf{Z}_2^j)}\right]\\
    &\overset{(a)}{=}-\mathbb E_\mathcal{Z}\log\left[\frac{\frac{p(\mathbf{Z}_1^i,\mathbf{Z}_2^i)}{p(\mathbf{Z}_1^i)p(\mathbf{Z}_2^i)}}{\sum_{j=0}^N\frac{p(\mathbf{Z}_1^j,\mathbf{Z}_2^j)}{p(\mathbf{Z}_1^j)p(\mathbf{Z}_2^j)}}\right] \\
    &=\mathbb E_\mathcal{Z}\log\left[1+\frac{p(\mathbf{Z}_1^i,\mathbf{Z}_2^i)}{p(\mathbf{Z}_1^i)p(\mathbf{Z}_2^i)}\sum_{j=1}^N\frac{p(\mathbf{Z}_1^j,\mathbf{Z}_2^j)}{p(\mathbf{Z}_1^j)p(\mathbf{Z}_2^j)}\right] \\
    &\approx \mathbb E_\mathcal{Z}\log\left[1+\frac{p(\mathbf{Z}_1^i,\mathbf{Z}_2^i)}{p(\mathbf{Z}_1^i)p(\mathbf{Z}_2^i)}N\mathbb E_{\mathbf{Z}_1}\left[\frac{p(\mathbf{Z}_1|\mathbf{Z}_2)}{p(\mathbf{Z}_1)}\right]\right] \\
    &= \mathbb E_\mathcal{Z}\log\left[1+\frac{p(\mathbf{Z}_1^i,\mathbf{Z}_2^i)}{p(\mathbf{Z}_1^i)p(\mathbf{Z}_2^i)}N\right] \\
    & \geq \log(N) - \mathbb E_\mathcal{Z}\log\left[\frac{p(\mathbf{Z}_1^i,\mathbf{Z}_2^i)}{p(\mathbf{Z}_1^i)p(\mathbf{Z}_2^i)}\right] \\
    &= \log(N) - \mathrm{I}(\mathbf{Z}_1;\mathbf{Z}_2).
\end{aligned}
\end{equation}
The equation (a) holds due to the Lemma \ref{lemma_1}. According to Eq.\ref{mutual}, we can derive $\mathrm{I}(\mathbf{Z}_1;\mathbf{Z}_2)\geq \log(N)-\mathcal{L}_{Z_1,Z_2}$. Similarly, we have the same conclusion for other views. Therefore, we have,
\begin{equation}
    \sum_{i\in\{w,p,e\}, j\in \{w,p,e\},i \neq j} \mathrm{I}(\mathbf{Z}_i;\mathbf{Z}_j) \geq 3\log(N) - \mathcal{L}_{cl}.
\end{equation}
We complete the proof of Theorem 1. Compared to the dual-view CL, we obtain a tighter lower bound on mutual information, as when CL loss is fully optimized, the first term on the right-hand side of the inequality becomes larger than before.

\subsection{A.3 Illustrative Explanation}
\label{explanation}
We present the illustrative explanation in Fig. \ref{picture}. When we only use the word-entity view, the mutual information of the pink part of the word-POS view and the cyan part of the POS-entity view is completely ignored, which potentially hinders model performance improvement.%When we only use the word-entity view, the mutual information of the red and cyan parts is completely ignored, which may improve the model performance.
\begin{figure}
    \centering
    \includegraphics[width=0.4\textwidth]{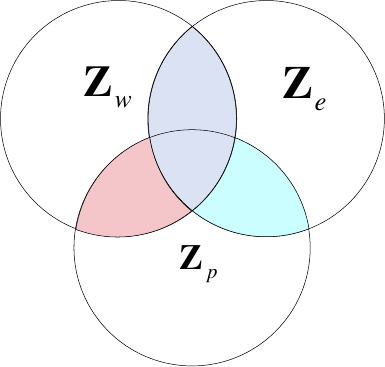}
    \caption{Diagram of mutual information under different views. $\mathbf{Z}_w, \mathbf{Z}_e$ and $\mathbf{Z}_p$ denote the embeddings learned from the word, tag, and entity views, respectively.}
    \label{picture}
\end{figure}
%Moreover, we also give the following corollary.

\subsection{A.4 Details of Baselines}
\label{details}
\textit{Modern Deep Learning Models}
\begin{itemize}
    \item \textbf{CNN} \cite{kim-2014-convolutional}: It adopts convolutional neural networks for feature extraction from texts, followed by classification based on the extracted features. 
    \item \textbf{LSTM} \cite{liu2015multi}: It utilizes long short-term memory neural networks to learn textual features, and subsequently constructs a classifier based on these features.
    \item \textbf{BERT} \cite{devlin2018bert}: It is a transformer-based model that utilizes bidirectional context to understand the meaning of words in a sentence.
    \item \textbf{RoBERTa} \cite{liu2019roberta}: It is a variant of BERT that optimizes the pretraining process and utilizes larger-scale data for better language representation learning.
\end{itemize}

\begin{table*}[ht]
\resizebox{0.95\textwidth}{!}{%
\begin{tabular}{@{}cl@{}}
\toprule
Dataset    & \multicolumn{1}{c}{Prompts}                                                                            \\ \midrule
Twitter       & Classify the tweets into negative or positive.                             \\ \midrule
MR         & Classify the movie reviews into negative or positive.                     \\ \midrule     
Snippets    & \begin{tabular}[c]{@{}l@{}}Classify the web search snippets into one of 8 classes: \{bussiness, computers, culture, education,\\ engineering, health, politics, sports\}.\end{tabular}  \\ \midrule
StackOverlow    & \begin{tabular}[c]{@{}l@{}}Classify the questions into one of 20 classes: \{svn, oracle, cocoa, visual-stdio, osx, wordpress, spring, \\hibernate, scala, sharepoint, ajax, drupal, qt, hashkell, linq, magento\}.\end{tabular}  \\ \midrule
\end{tabular}%
}
\caption{Examples of prompts used for different datasets.}
\label{prompts}
\end{table*}

\noindent \textit{Graph-Based Models}
\begin{itemize}
    \item \textbf{TLGNN} \cite{huang2019text}: It creates a graph for each document and conducts graph convolution operations to capture multi-hop word interactions.
    \item \textbf{HyperGAT} \cite{ding2020more}: It employs a hypergraph to depict each document and executes hypergraph attention operations to acquire embeddings that encompass higher-order word interactions.
    \item \textbf{TextING} \cite{zhang2020every}: It creates separate graphs for each text and utilizes gated GNNs to integrate neighboring information.
    \item \textbf{DADGNN} \cite{liu2021deep}: It has the capability to capture contextual information and separates the two processes of GNNs by utilizing an attention diffusion mechanism, allowing for the training of deeper neural networks.
    \item \textbf{TextGCN} \cite{yao2019graph}: It performs vanilla GCNs on the given texts to extract expressive features, and then proceeds with the classification task.
\end{itemize}

\noindent \textit{Deep Short Text Models}
\begin{itemize}
    \item \textbf{STCKA} \cite{chen2019deep}: It leverages the provided knowledge base to integrate factual information and improve the semantic representations of the text.
    \item \textbf{STGCN} \cite{ye2020document}: It utilizes a corpus-level graph and integrates word embeddings acquired by GNNs with word embeddings generated by pre-trained BERT using a BiLSTM model.
    \item \textbf{HGAT} \cite{linmei2019heterogeneous}: It utilizes a heterogeneous information network to seamlessly integrate various forms of supplementary information through the use of node-level and type-level attention mechanisms.
    \item \textbf{SHINE} \cite{wang2021hierarchical}: It constructs a hierarchical graph and dynamically learns short text graphs to make inferences about unlabeled texts using the learned structural information.
    \item \textbf{NC-HGAT} \cite{su2022contrastive}: It is built on top of HGAT and performs CL by perturbing the constructed text graph to learn more informative text representations.
    \item \textbf{GIFT} \cite{liu2024improved}: It first obtains the augmented text view by performing SVD on the word-document matrix, and then conducts graph contrastive learning on the two text views. 
\end{itemize}

\noindent \textit{Large Language Models}
\begin{itemize}
    \item \textbf{GPT-3.5} \cite{ouyang2022training}: It adopts decoder-only architecture and reinforcement learning from human feedback techniques to continuously fine-tune the pre-trained model, aiming to enhance the model understanding of human instructions.
    \item \textbf{Bloom-7.1B} \cite{workshop2022bloom}: It also utilizes a decoder-only architecture, is trained on a cross-linguistic corpus with multi-task prompts, demonstrating improved performance across many natural language tasks.
    \item \textbf{Llama2-7B} \cite{touvron2023llama}: It is a language model based on a decoder Transformer architecture, trained on a novel amalgamation of data from public datasets, which enlarges the pretraining corpus by 40\%, doubles the model context length, and employs grouped query attention.
    \item  \textbf{Llama3-8B} \cite{llama3modelcard}: It uses the same model architecture as Llama2, with the main difference being that it is pre-trained on over 150 trillion tokens from public data sources.
\end{itemize}

\subsection{A.5 Implementation Details of Baselines}
\label{implementation}
For CNN and LSTM, we uniformly initialize word embeddings using pre-trained GloVe embeddings and then train them with neural networks. As for BERT and RoBERTa, pre-trained language models on large corpus, we fine-tune them along with the subsequent classifier using the target dataset. For graph-based and deep short text models, we use the original implementations and the default hyperparameters suggested by the works. We present the used prompts in Table \ref{prompts}.

%For large language models, we fine-tune GPT-3.5 using the fine-tuning interface provided by OpenAI with the training data from the evaluation dataset, and obtain the results based on the prompts in Table \ref{prompts}. For Bloom-7.1B and Llama2-7B, we conduct full-scale fine-tuning using the training data. To reduce GPU memory usage, we adopt the Parameter Efficient Fine-Tuning (PEFT) method with LoRA and 4-bit quantization techniques provided by Hugging Face. The prompts used for STC in Bloom-7.1B and Llama2-7B are the same as those used in GPT-3.5.

%We fine-tune GPT-3.5 using OpenAI's fine-tuning interface with the training data from the evaluation dataset and obtain results based on the prompts in Table \ref{prompts}. Additionally, for Bloom-7.1B, Llama2-7B, and Llama3-8B, we conduct comprehensive fine-tuning using the training data. To reduce GPU memory usage, we employ the Parameter Efficient Fine-Tuning (PEFT) method with LoRA and 4-bit quantization techniques provided by Hugging Face. The prompts used for STC in Bloom-7.1B, Llama2-7B, and Llama3-8B are the same as those used in GPT-3.5.

%\noindent \textbf{Experimental Environment}: We use the PyTorch library 1.10 to implement our model with Python 3.7. Moreover, we adopt the NVIDIA RTX 3090Ti GPU to accelerate the model training.

\subsection{Performance on Long and Unstructed Texts}
\label{long_text}
To further demonstrate the superiority of our proposed model, in addition to our primarily focused on short-text classification tasks, we also attempt to apply SimSTC to long-text datasets \textbf{R52} \cite{yao2019graph} and \textbf{AG\_news} \cite{zhang2015character}, as well as unstructured datasets \textbf{SST-5} \cite{socher2013recursive} and \textbf{CR} \cite{ding2008holistic}. We present the experimental results of our proposed model and several selected powerful baselines in Table \ref{res_sup}. The statistics of these datasets are presented in Table \ref{dataset_sup}.

\begin{table}[ht]
\resizebox{0.49\textwidth}{!}{%
\begin{tabular}{@{}c|cccc@{}}
\toprule
Dataset  & \#Doc   & \#Train(ratio) & Avg.Length & \#Class \\ \midrule
R52      & 9,100   & 1040(11.43\%)  & 69.82      & 52      \\
AG\_news & 127,600 & 80(0.06\%)     & 44.03      & 4       \\
SST-5    & 11,855  & 100(0.84\%)    & 20.17      & 5       \\
CR       & 3,775   & 40(1.06\%)           & 19         & 2       \\ \bottomrule
\end{tabular}%
}
\caption{Statistics of the additional datasets.}
\label{dataset_sup}
\end{table}

\begin{table*}[h]
\resizebox{\textwidth}{!}{%
\begin{tabular}{@{}c|cccccccc@{}}
\toprule
\multirow{2}{*}{Model} & \multicolumn{2}{c}{R52} & \multicolumn{2}{c}{AG\_news} & \multicolumn{2}{c}{SST-5} & \multicolumn{2}{c}{CR}  \\ \cmidrule(l){2-9} 
                       & ACC        & F1         & ACC           & F1           & ACC         & F1          & ACC        & F1         \\ \midrule
TextING                & 91.20$\pm$0.19 & 90.20$\pm$0.70 & 91.22$\pm$0.39    & 90.66$\pm$0.23   & 43.10$\pm$0.23  & 42.65$\pm$0.29  & 85.32$\pm$0.31 & 84.36$\pm$0.27 \\
DADGNN                 & 92.15$\pm$0.22 & 89.36$\pm$0.42 & 90.40$\pm$0.32    & 89.86$\pm$0.22   & 45.15$\pm$0.26  & 42.96$\pm$0.32  & 86.29$\pm$0.09 & 85.10$\pm$0.23 \\
TextGCN                & 93.56$\pm$0.29 & 91.80$\pm$0.92 & 90.84$\pm$0.29    & 89.99$\pm$0.30   & 40.65$\pm$0.06  & 39.92$\pm$0.16  & 84.32$\pm$0.21 & 86.51$\pm$0.29 \\
SHINE                  & 82.79$\pm$0.39 & 82.35$\pm$0.36 & 87.95$\pm$0.22    & 86.89$\pm$0.15   & 44.39$\pm$0.21  & 41.62$\pm$0.22  & 79.05$\pm$0.52 & 78.73$\pm$0.29 \\
NC-HGAT                & 81.76$\pm$0.35 & 79.96$\pm$0.29 & 86.46$\pm$0.22    & 85.14$\pm$0.20   & 43.42$\pm$0.22  & 42.19$\pm$0.26  & 77.59$\pm$0.32 & 76.06$\pm$0.30 \\ \midrule
Bloom-7.1B               & 93.52$\pm$0.45 & 90.56$\pm$0.26 & 92.03$\pm$0.15    & 90.96$\pm$0.19   & 51.39$\pm$0.29  & 50.76$\pm$0.32  & 91.40$\pm$0.53 & 90.65$\pm$0.31 \\
Llama2-7B              & 94.45$\pm$0.22 & 93.40$\pm$0.22 & 91.26$\pm$0.19    & 90.29$\pm$0.21   & 52.05$\pm$0.22  & 51.15$\pm$0.25  & 92.29$\pm$0.50 & 91.56$\pm$0.29 \\ 
Llama3-8B              & 94.96$\pm$0.36 & 93.96$\pm$0.39 & 93.22$\pm$0.29    & 92.09$\pm$0.26   & 53.25$\pm$0.26  & 52.15$\pm$0.55  & 92.99$\pm$0.52 & 92.25$\pm$0.32 \\ \midrule
SimSTC                 & \textbf{95.56$\pm$0.39} & \textbf{95.40$\pm$0.15} & \textbf{93.56$\pm$0.12}    & \textbf{92.30$\pm$0.12}   & \textbf{54.24$\pm$0.32}  & \textbf{53.14$\pm$0.25}  & \textbf{93.07$\pm$0.26} & \textbf{92.98$\pm$0.25} \\ \bottomrule
\end{tabular}%
}
\caption{Results (\%) of the accuracy and macro-F1 score on several additional text datasets.}
\label{res_sup}
\end{table*}

Based on the above results, it is evident that our model demonstrates outstanding performance even on extended and unstructured datasets. This outcome serves as compelling evidence of the scalability and robustness of our approach.
